# Supplementary material for: Through the Theory of Mind's Eye: Reading Minds with Multimodal Video Large Language Models
Source: arXiv:2406.13763 source file (2025-09-15)
Supplement: Supplementary file 1 [file appendix_exampletrajectories.tex]

\section{Qualitative Comparisons of Different Credit Assignment Methods} \label{app:credit_assignment_qualitative}
We present qualitative comparison results of different credit assignment in \autoref{fig:qualitative}. First of all, we observe that LLM-as-a-Judge can easily get distracted by the length and format of the response without actually attending to its utility for task success. Furthermore, while being a natural practice in deep RL literature, the use of a value function fails to reasonably predit the expected future utility in unseen tasks. In particular, it predicts that the first candidate response has a probability of \emph{97\%} to lead to the final success of the agent despite being only the second turn out of 10 turns and this candidate response being phrased in a very confusing way. In contrast, \methodname{} is able to tell the advantage of the second response with a higher score because it is important in this task for the agent to figure out that the returned list can contain duplicate objects. This shows the importance of the RL algorithmic choices of \methodname{} and that the go-to practice of training a value function may generalize arbitrarily poorly in unseen tasks.

\begin{figure*}[!h]
     \centering
    \includegraphics[width=0.8\textwidth]{figures/qualitative_comparisons.pdf}
        \caption{\textbf{Qualitative comparisons between different credit assignment methods.} A fixed LLM-as-a-Judge can be easily distracted by length and formats of the actions without considering their actual utility. A value function generalizes poorly to unseen tasks. In contrast, SWEET can attend to the actual utility of the action for task success and generalize well.}
        \label{fig:qualitative} 
        \vspace{-0.5cm}
\end{figure*}

\section{Full Qualitative Examples} \label{app:full_qualitative}
To demonstrate the level of difficulty of tasks in \benchmarkname{} and provide a qualitative comparisons of different models, we have included examples of full trajectories in this section. 

In particular, in \autoref{fig:backend_ours_qualiatative}, \autoref{fig:backend_ours_continued_qualiatative}, \autoref{fig:backend_zeroshot}, \autoref{fig:backend_gpt4o}, we have provided full trajectories on Backend Programming for \methodname{} Llama-3.1-8B-Instruct, Zeroshot Llama-3.1-8B-Instruct, and Zeroshot GPT4-O. While zeroshot baselines do try to propose some critical questions to seek more information from the human collaborator, they quickly jump into conclusions without gathering enough information, thus resulting in a wrong answer. Such failure modes exist even for stronger general-purpose LLMs like GPT4-O, indicating that task-specific tuning may always be necessary despite the improvement in the capability of the base model. In contrast, \methodname{} Llama-3.1-8B-Instruct learnt back-and-forth information-seeking behaviors and only answered the question once all information has been collected. Surprisingly, we found that RL training also results in some emergent behaviors such as reasoning with longer chain-of-thought and even self-corrections as shown in the last response from the agent in \autoref{fig:backend_ours_continued_qualiatative}.

We also include a full trajectory example on Frontend Design with \methodname{} Llama-3.1-8B-Instruct in \autoref{fig:frontend_1}, \autoref{fig:frontend_2}, \autoref{fig:frontend_3}, \autoref{fig:frontend_4}, \autoref{fig:frontend_5}, \autoref{fig:frontend_6}. We would like to note the significant complexity of this task where the agent needs to reason about HTML code over an extended horizon (up to 16k tokens), as a HTML code snippet is included in the response of each turn. After \methodname{} training, the LLM agent has learnt nuanced collaborative and reward-maximizing behaviors where it first proposes a scratch solution to gather coarse-grained feedback and only perform fine-grained edits in the end.

\begin{figure*}[!h]
     \centering
     \vspace{-0.3cm}
    \includegraphics[width=.95\textwidth]{figures/backend_ours.pdf}
        \caption{\footnotesize{\textbf{Example full trajectory for Backend Programming with \methodname{} Llama-3.1-8B-Instruct.} After training, the LLM agent has learnt back-and-forth information seeking behaviors before giving the final answer. }}
        \label{fig:backend_ours_qualiatative} 
\end{figure*}

\begin{figure*}[!h]
     \centering
     \vspace{-0.3cm}
    \includegraphics[width=.95\textwidth]{figures/backend_ours_continued.pdf}
        \caption{\footnotesize{\textbf{Example full trajectory for Backend Programming with \methodname{} Llama-3.1-8B-Instruct (Continued).} After training, the LLM agent has learnt back-and-forth information seeking behaviors before giving the final answer. }}        \label{fig:backend_ours_continued_qualiatative} 
\end{figure*}

\begin{figure*}[!h]
     \centering
    \includegraphics[width=.95\textwidth]{figures/backend_zeroshot.pdf}
        \caption{\footnotesize{\textbf{Example full trajectory for Backend Programming with Zeroshot Llama-3.1-8B-Instruct.} While the agent has asked a few questions, it quickly jumps into conclusions, resulting in a wrong final answer.}}
        \label{fig:backend_zeroshot} 
\end{figure*}

\begin{figure*}[!h]
     \centering
    \includegraphics[width=.95\textwidth]{figures/backend_gpt4o.pdf}
        \caption{\footnotesize{\textbf{Example full trajectory for Backend Programming with Zeroshot GPT-4O.} While the agent does propose critical questions to the human collaborator, it also has the issue of jumping into conclusions.}}
        \label{fig:backend_gpt4o} 
\end{figure*}

\begin{figure*}[!h]
     \centering
    \includegraphics[width=.95\textwidth]{figures/frontend_ours_1.pdf}
        \caption{\footnotesize{\textbf{Example full trajectory for Frontend Design with \methodname{} Llama-3.1-8B-Instruct (1).} After training, the LLM agent has learnt sophisticated task-specific strategies to optimize the final reward.}}
        \label{fig:frontend_1} 
\end{figure*}

\begin{figure*}[!h]
     \centering
    \includegraphics[width=.95\textwidth]{figures/frontend_ours_2.pdf}
        \caption{\footnotesize{\textbf{Example full trajectory for Frontend Design with \methodname{} Llama-3.1-8B-Instruct (2).} After training, the LLM agent has learnt sophisticated task-specific strategies to optimize the final reward.}}
        \label{fig:frontend_2} 
\end{figure*}

\begin{figure*}[!h]
     \centering
    \includegraphics[width=.95\textwidth]{figures/frontend_ours_3.pdf}
        \caption{\footnotesize{\textbf{Example full trajectory for Frontend Design with \methodname{} Llama-3.1-8B-Instruct (3).} After training, the LLM agent has learnt sophisticated task-specific strategies to optimize the final reward.}}
        \label{fig:frontend_3} 
\end{figure*}

\begin{figure*}[!h]
     \centering
    \includegraphics[width=.95\textwidth]{figures/frontend_ours_4.pdf}
        \caption{\footnotesize{\textbf{Example full trajectory for Frontend Design with \methodname{} Llama-3.1-8B-Instruct (4).} After training, the LLM agent has learnt sophisticated task-specific strategies to optimize the final reward.}}
        \label{fig:frontend_4} 
\end{figure*}

\begin{figure*}[!h]
     \centering
    \includegraphics[width=.95\textwidth]{figures/frontend_ours_5.pdf}
        \caption{\footnotesize{\textbf{Example full trajectory for Frontend Design with \methodname{} Llama-3.1-8B-Instruct (5).} After training, the LLM agent has learnt sophisticated task-specific strategies to optimize the final reward.}}
        \label{fig:frontend_5} 
\end{figure*}

\begin{figure*}[!h]
     \centering
    \includegraphics[width=.95\textwidth]{figures/frontend_ours_6.pdf}
        \caption{\footnotesize{\textbf{Example full trajectory for Frontend Design with \methodname{} Llama-3.1-8B-Instruct (6).} After training, the LLM agent has learnt sophisticated task-specific strategies to optimize the final reward.}}
        \label{fig:frontend_6} 
\end{figure*}
