# Supplementary material for: Through the Theory of Mind's Eye: Reading Minds with Multimodal Video Large Language Models
Source: arXiv:2406.13763 source file (2025-09-15)
Supplement: Supplementary file 2 [file appendix_hyperparameters.tex]

\section{Hyperparameters}
For completeness and reproducibility, we present all hyperparameters used in \methodname{} and all baselines in \autoref{tab:hyperparametersZZ}. In general, we found that the performances of both Multi-Turn DPO and SWEET-RL are consistent with respect to the hyperparameters in the DPO loss objective such as learning rate and beta, and the inclusion of a negative-log-likelihood coefficient of 0.01 helps in most cases (\citet{pang2024iterativereasoningpreferenceoptimization} also found this to be useful).

\begin{table}[h] 
\centering
\caption{Hyperparameters for \methodname{} and baseline methods for all experiments.}
\label{tab:hyperparametersZZ}
\resizebox{.8\linewidth}{!}{  
\begin{tabular}{c|c|cc} 
\toprule
& & Backend Programming& Frontend Design \\
\hline
\multirow{2}{8em}{Rejection Fine-Tuning} & learning rate & 2e-7 & 2e-7\\
& batch size& 32 & 32 \\
& epochs & 4 & 8 \\
\hline
\multirow{4}{8em}{Multi-Turn DPO} & learning rate & 2e-7 & 2e-7\\
& beta & 0.1 & 0.1\\
& negative-log-likelihood loss coefficient & 0.01 & 0.01\\
& batch size& 8 & 8 \\
& epochs & 4 & 8 \\
\hline
\multirow{8}{8em}{\methodname} & critic learning rate & 2e-7 & 2e-7\\
& critic beta & 0.1 & 0.1\\
& critic negative-log-likelihood loss coefficient & 0.01 & 0.01\\
& critic batch size& 8 & 8 \\
& critic epochs & 4 & 8 \\
& actor lr & 2e-7 & 2e-7\\
& actor beta & 0.1 & 0.1\\
& actor negative-log-likelihood loss coefficient & 0.01 & 0.01\\
& actor batch size& 8 & 8\\
& actor epochs & 1 & 1 
\end{tabular}}
\end{table}
