# Supplementary material for: Through the Theory of Mind's Eye: Reading Minds with Multimodal Video Large Language Models
Source: arXiv:2406.13763 source file (2025-09-15)
Supplement: Supplementary file 3 [file appendix_prompts.tex]

\section{Prompts}
For completeness, we have included the prompt that we used for testing different models on Backend Programming in ~\autoref{fig:backend-prompt} and on Frontend Programming in ~\autoref{fig:frontend-prompt}.

\begin{figure}
    \centering
    \setlength{\fboxrule}{0.5pt}
    \fbox{
        \parbox{.95\textwidth}{
            \textbf{Backend Programming Prompt}\\
You are a helpful LLM agent. 

Your task is to help a human user to resolve their problem, in particular python programming.

1) Note that the problem is highly personalized so you need to explicitly gather information by asking questions to the human user about some hidden information and implicit constraints.

YOU SHOULD TRY TO ASK CLARIFICATION QUESTIONS.

2) Note that you should not ask human users complicated questions as they will only answer questions briefly in two sentences.

3) When you have gathered enough information to answer, say "I WANT TO ANSWER:" in the beginning of your response and provide your final answer.

4) Note that you can only interact with the human users WITHIN 10 back-and-forth rounds and you have to provide your final answer before the conversation ends.

5) You should be as concise as possible in your response to human.

"I WANT TO ANSWER:" should be included in your response to human if you think that you have gathered enough information for addressing this problem.

Directly output the raw python code after "I WANT TO ANSWER:".

Complete only the immediate agent response in this dialogue:
        }
    }
    \caption{\textbf{The prompt used for testing different models on Backend Programming task.}}
    \label{fig:backend-prompt}
\end{figure}

\begin{figure}
    \centering
    \setlength{\fboxrule}{0.5pt}
    \fbox{
        \parbox{.95\textwidth}{
            \textbf{Frontend Design Prompt}\\
You are a helpful LLM agent. 
Your task is to help a human user to code a complete website with a good design in HTML and Tailwind CSS.
Write the code inside a tag <html>.
Write real and long sentences about the business.
You don’t have to include images, but if you do, use only this source
https://picsum.photos/id/48/W/H, by replacing W and H with the width and height of the image.
Keep the id the same to only use id 48 image.

1) Note that the problem is highly personalized so you need to go through a few rounds of revisions.

2) When you have gathered enough information to answer, say "I WANT TO ANSWER:" in the beginning of your response and provide your final answer.

3) Note that you can only interact with the human users WITHIN 10 back-and-forth rounds and you have to provide your final answer before the conversation ends.

4) You will be judged both by the quality of the final answer and the efficiency of the conversation.

5) You can include ONLY ONE snippet raw html and Tailwind css code (wrapped in html tag)in your response to human user to ask how is the proposed design different from what the human user wants. 
This snippet of raw html and Tailwind css code (WRAPPED IN html TAG) will be rendered for the human to see a screenshot of the webpage. The human user will respond by comparing your rendered webpage with the webpage that the human user has in mind.

6) You need to make sure that your html webpage looks exactly as the human user wants, including the overall layout, navigation bars, background color etc.

7) The human user can only see your rendered image and provide suggestions based on the rendered image, and not any text questions.

First output your thought on your remaining uncertainties about the understanding of the problem and user preferences such as name of the function, input format, output format, and etc.
Then say "OUTPUT:\\n" followed by your proposal html.
        }
    }
    \caption{\textbf{The prompt used for testing different models on Frontend Design task.}}
    \label{fig:frontend-prompt}
\end{figure}
