# Supplementary material for: Through the Theory of Mind's Eye: Reading Minds with Multimodal Video Large Language Models
Source: arXiv:2406.13763 source file (2025-09-15)
Supplement: Supplementary file 4 [file appendix_proofs.tex]

\section{Theoretical Justifications} \label{app:theory}
In this section, we will provide some theoretical justifications for the derivation of our method. We first show that the trajectory-level Bradley-Terry objective can be similarly used for learning the advantage function:

\begin{lemma}\label{lem:rA}
    For an MDP with each state $(o,c) \in \mathcal{O} \times \mathcal{C}$ and for any $\pi: \mathcal{O} \mapsto \mathcal{A}$, assume the transition function $\mathcal{T}(o, a, c)$ is deterministic for any $(o, a, c)$ then the following holds $\forall \tau^+, \tau^-$:
\begin{align*}
    -\log \left[\sigma\left(\sum_{t} \beta r(o^+_t, a^+_t, c) - \sum_{t} \beta r(o^-_t, a^-_t, c)\right)\right] = -\log \left[\sigma\left(\sum_{t} \beta A^\pi(o^+_t, a^+_t, c) - \sum_{t} \beta A^\pi(o^-_t, a^-_t, c)\right)\right]
\end{align*}
\end{lemma}
\begin{proof}
    To show this, we would like to prove:
    \begin{align*}
        \sum_{t} r(o_t, a_t, c) = \sum_t A^\pi(o_t, a_t, c)
    \end{align*}
    We will prove this by telescoping:
    \begin{align*}
        & \sum_t A^\pi(o_t, a_t, c)\\
        = & \sum_t \left[Q^\pi(o_t, a_t, c) - V^\pi(o_t, c) \right]\\
        = & \sum_{t=1}^{N-1} \left[r(o_t, a_t, c) + \mathbb{E}_{o'_{t+1} \sim \mathcal{T}(\cdot|o_t, a_t, c)} V^\pi(o'_{t+1}, c) - V^\pi(o_t, c) \right]  + r(o_N, a_N, c)\\
        = & \sum_{t=1}^{N} r(o_t, a_t, c) + \sum_{t=1}^{N-1}\left[\mathbb{E}_{o'_{t+1} \sim \mathcal{T}(\cdot|o_t, a_t, c)} V^\pi(o'_{t+1}, c) - V^\pi(o_t, c) \right] \\
        = & \sum_{t=1}^{N} r(o_t, a_t, c),
    \end{align*}
    where the last equality follows by the assumption of deterministic transition.
\end{proof}

Additionally, we would like to also provide a theoretical justification for using an asymmetric critic for optimizing the actor with a different observation space. Intuitively, although for each sample such a training-time advantage function may give a different judgement compared to its regular counterpart, the following lemma shows that the policy gradient~\citep{Williams2004SimpleSG} estimated from an advantage function with training-time information is unbiased averaged over all samples. 

\begin{lemma}\label{lem:unbiased}
    For an MDP with each state $(o,c) \in \mathcal{O} \times \mathcal{C}$ and for any $\pi: \mathcal{O} \mapsto \mathcal{A}$, let $d^\pi_t(o_t, a_t, c)$ to be joint state-action occupancy distribution at step $t$, the following two estimators are both unbiased estimators of the policy gradient of $\pi$:
\begin{align*}
    \nabla \mathbb{E}_{\tau \sim \pi} \left(\sum_{t=1}^H r(o_t, a_t, c) \right) =& \sum_{t=1}^N \mathbb{E}_{o_t, a_t} A^\pi(o_t,a_t) \nabla \log \pi(a_t|o_t) 
    = \sum_{t=1}^N \mathbb{E}_{o_t,a_t, c} A^\pi(o_t,a_t, c) \nabla \log \pi(a_t|o_t)
\end{align*}
\end{lemma}

\begin{proof}
    The proof of this lemma is similar to the standard policy gradient analysis~\citep{agarwal2019reinforcement}.
    \begin{align*}
         \nabla \mathbb{E}_{\tau \sim \pi} \left(\sum_{t=1}^N r(o_t, a_t, c) \right) 
        = & \nabla \EE_{c} \mathbb{E}_{o_1} V^\pi(o_1)\\
        = & \EE_{c} \mathbb{E}_{o_1} \nabla V^\pi(o_1)\\
        = & \EE_{c} \mathbb{E}_{o_1} \nabla  \left[\sum_{a_1} \pi(a_1|o_1) Q^\pi(o_1, a_1)\right] \\
        = & \EE_{c} \mathbb{E}_{o_1} \left[\sum_{a_1} (\nabla \pi(a_1|o_1)) Q^\pi(o_1, a_1) + \sum_{a_1}\pi(a_1|o_1) \nabla Q^\pi(o_1, a_1) \right]\\
        = & \EE_{c} \mathbb{E}_{o_1} \left[\sum_{a_1} \pi(a_1|o_1) (\nabla \log\pi(a_1|o_1)) Q^\pi(o_1, a_1) + \sum_{a_1}\pi(a_1|o_1) \nabla Q^\pi(o_1, a_1) \right] \\
        = & \EE_{c} \mathbb{E}_{o_1} \left[\EE_{a_1} (\nabla \log\pi(a_1|o_1)) Q^\pi(o_1, a_1) + \sum_{a_1}\pi(a_1|o_1) \nabla Q^\pi(o_1, a_1) \right] \\
        = & \EE_{c} \mathbb{E}_{o_1} \left[\EE_{a_1} (\nabla \log\pi(a_1|o_1)) Q^\pi(o_1, a_1) + \EE_{a_1} \EE_{o_2}\nabla V^\pi(o_2) \right] \\
        = & \EE_{c} \sum_{t=1}^N \EE_{o_t, a_t} Q^\pi(o_t, a_t) \nabla \log \pi(a_t|o_t).
    \end{align*}
    To proceed, we need to first show a useful equality:
    \begin{align*}
        \EE_{o_t, a_t} V^\pi(o_t) \nabla \log \pi(a_t|o_t)
        = & \EE_{o_t} \sum_a \pi(a_t|o_t) V^\pi(o_t) \nabla \log \pi(a_t|o_t)\\
        = & \EE_{o_t} \sum_a V^\pi(o_t) \nabla \pi(a_t|o_t)\\
        = & \EE_{o_t}  V^\pi(o_t) \nabla \sum_a \pi(a_t|o_t)\\
        = & \EE_{o_t}  V^\pi(o_t) \nabla 1\\
        = &0
    \end{align*}
    Therefore, we can use the advantage function instead of the $Q$-function in the expression of policy gradients:
    \begin{align*}
         \nabla \mathbb{E}_{\tau \sim \pi} \left(\sum_{t=1}^N r(o_t, a_t, c) \right) 
         = & \EE_{c} \sum_{t=1}^N \EE_{o_t, a_t} Q^\pi(o_t, a_t) \nabla \log \pi(a_t|o_t)\\
         = & \EE_{c} \sum_{t=1}^N \EE_{o_t, a_t} (Q^\pi(o_t, a_t) - V^\pi(o_t, a_t)) \nabla \log \pi(a_t|o_t)\\
         = & \EE_{c} \sum_{t=1}^N \EE_{o_t, a_t} A^\pi(o_t, a_t) \nabla \log \pi(a_t|o_t)\\
         = & \sum_{t=1}^N \EE_{o_t, a_t}  \left(\nabla \log \pi(a_t|o_t)\right) \EE_{c}  A^\pi(o_t, a_t)\\
         = & \sum_{t=1}^N \EE_{o_t, a_t}  \left(\nabla \log \pi(a_t|o_t)\right) \EE_{c}  A^\pi(o_t, a_t, c)\\
         = & \EE_{c} \sum_{t=1}^N \EE_{o_t, a_t}  \left(\nabla \log \pi(a_t|o_t)\right)   A^\pi(o_t, a_t, c),
    \end{align*}
    where the second last equation follows from the fact that $\EE_{c \sim d^\pi_t(\cdot|o_t, a_t)} A^\pi(o_t, a_t, c) = A^\pi(o_t, a_t)$.
\end{proof}
